# Supplementary material for: Reconfigurable random bit storage using polymer-dispersed liquid crystal
Source: arXiv:1403.2419 ancillary file (2014-03-10)
Supplement: Supplementary file 1 [file Supplementary_text.pdf]

# Reconfigurable random bit storage using polymer-dispersed liquid crystal: Supplementary information

**R. Horstmeyer, S. Assawaworrarit and C. Yang**

## Supplementary Section 1: Randomness Test Performance

As described in the main text, our ROSS key set is generated through the following steps: 1) detect a sequence of uncorrelated speckle intensity images, 2) unwrap each image into a 1D vector, 3) multiply each of these vectors by the random matrix projection operator $\boldsymbol{H}$, 4) concatenate the results of these matrix multiplications into a single vector, comprising the key set. These four steps are sequentially explained in the following three sections. Before getting into details, we first demonstrate that the end product of the ROSS device is indeed statistically random and hence suitable as a random bit source (and secure storage mechanism) for nearly any cryptographic application.

Without a specific way to define ideal randomness for a finite sequence of bits, robust and thorough statistical testing is well recognized as the optimal method of checking the effectiveness of a random number generation procedure [1-3]. We test our ROSS key set's statistical randomness using both the Diehard [1] and NIST [2, 3] random number generator test suites. These statistical tests consist of establishing a null hypothesis of whether or not the tested

**Supplementary Table 1**: **Statistics of ROSS keys from NIST randomness tests**

| Statistical Test | p-value$^+$ | Proportion | Pass/Fail |
|---|---|---|---|
| Frequency | 0.069 | 0.9948 | Pass |
| Block Frequency | 0.065 | 0.9948 | Pass |
| Cumulative Sums | 0.482$^+$ (2) | 0.9896 | Pass |
| Runs | 0.310 | 0.9792 | Pass |
| Longest Run | 0.016 | 0.9792 | Pass |
| Rank | 0.350 | 0.9896 | Pass |
| FFT | 0.452 | 0.9896 | Pass |
| Non-overlapping Template | 0.009$^+$ (147) | 0.9688 | Pass |
| Overlapping Template | 0.734 | 0.9948 | Pass |
| Universal | 0.042 | 0.9896 | Pass |
| Approximate Entropy | 0.180 | 0.9844 | Pass |
| Random Excursions | 0.014$^+$ (8) | 0.9832 | Pass |
| Random Excursions Variant | 0.081$^+$ (18) | 0.9748 | Pass |
| Serial | 0.811$^+$ (2) | 0.9948 | Pass |
| Linear Complexity | 0.620 | 1.0000 | Pass |

**Supplementary Table 1 | Example NIST statistical randomness test performance.** NIST statistical randomness test suite performance of an arbitrarily selected 24 MB sequence of ROSS key data. All keys were grouped together, then split into 192 unique 1 megabit sequences following prior test methods [4-5]. For 'success' using 192 samples of $10^6$ bit sequences and significance level $\alpha$ =0.01, the p-value (uniformity of p-values) should be larger than 0.001 and the minimum pass rate is 0.968458. Tests that produce multiple p-values and proportions are denoted by a ($^+$), followed by the number of different test values generated in parenthesis. The table displays the lowest (i.e., worst-case) generated p-values and proportions in the set.

sequence exhibits mathematical properties consistent with a random bit sequence, and then checking within a given level of significance if the null hypothesis is verified.

Since we eventually use fuzzy commitment to ensure our keys are error-free (see Section 3), the initially generated key set is split into two components: a code that forms the random keys, and a witness to hide the digitally saved code. We note here that the below statistical tests are performed on example 24 MB key sets before this split, thus verifying the statistical randomness of both the code and witness components for fuzzy commitment. For the NIST test (Supplementary Table 1), we split the 24 MB key sets into 192 unique 1 megabit sequences following prior test methods [4-5]. The entire 24 MB key was input for the Diehard test (Supplementary Table 2). All statistical tests in both test packages are satisfied assuming a statistical significance level of $\alpha$= 0.01, as used elsewhere [4, 5]. In total, the NIST and Diehard tests were repeated on four different 24 MB data sequences for 2 unique ROSS setups. All independent test results followed similar statistics as those presented in the following two tables.

**Supplementary Table 2**: **Statistics of ROSS keys from Diehard randomness tests**

| **Statistical Test** | **p-value$^{+}$** | **Pass/Fail** | **KS** |
|---|---|---|---|
| Birthday Spacings | 0.887 | Pass | Y |
| Overlapping Permutations | 0.473 | Pass | |
| Ranks of $31^2$ Matrices | 0.615 | Pass | |
| Ranks of $32^2$ Matrices | 0.123 | Pass | |
| Ranks of 6x8 Matrices | 0.046 | Pass | Y |
| Bitstream Test | $0.022^{+}$ (18) | Pass | |
| Overlapping Pairs, Sparse Occupancy | $0.019^{+}$ (22) | Pass | |
| Overlapping-Quadruples-Sparse-Occupancy | $0.018^{+}$ (27) | Pass | |
| DNA | $0.066^{+}$ (29) | Pass | |
| Count the 1`s | 0.403 | Pass | |
| Count the 1`s in Specific Bytes | $0.093^{+}$ (25) | Pass | |
| Parking Lot Test | 0.230 | Pass | Y |
| Minimum Distance Test | 0.574 | Pass | Y |
| Random Spheres Test | 0.532 | Pass | Y |
| The Squeeze Test | 0.433 | Pass | |
| Overlapping Sums Test | 0.291 | Pass | Y |
| Runs Test | 0.268 | Pass | Y |
| Craps Test | 0.568 | Pass | |

**Supplementary Table 2 | Example Diehard statistical randomness tests performance.** Diehard Random Test Suite performance for the same sequence of 24 MB of ROSS key data (concatenated into a single vector) as used in the NIST tests in Supplementary Table 1. A p-value > 0.0001 indicates a significance level of $\alpha$= 0.01, which is typically considered passing [4,5]. Tests using the Komolgorov-Smirnov (KS) test to obtain a single statistical p-value are denoted with a "Y" in the last column. The lowest p-value is displayed for tests that generate multiple p-values without using the KS test. These tests are denoted with a ($^{+}$) after their p-value, followed by the number of tests used in parenthesis.

## Supplementary Section 2: Digital Whitening

Many "whitening" procedures exist to convert a biased random bit sequence into an unbiased and uncorrelated bit stream [6-9]. We adopt the linear randomness extraction operation proposed in [10] to turn each of our detected speckle vectors $\boldsymbol{s}$ (which contain both biased and slightly correlated pixels) into a random key vector $\boldsymbol{k}$. This linear operation is performed as a sparse binary random matrix multiplication. One large sparse random matrix $\boldsymbol{H}$ is constructed using a pseudo-random number generator and then saved digitally within each ROSS device (approximately $10^{12}$ matrix entries, with $10^8$ non-zero entries). We assume this matrix is publically known and may be accessed by an attacker without any loss of security. Its contained randomness adds no entropy to the random key $\boldsymbol{k}$. Instead, its randomized construction simply facilitates efficient entropy extraction from each biased, weakly random speckle vector $\boldsymbol{s}$.

In the presented work, the number of columns in $\boldsymbol{H}$ matches the length of each speckle vector $\boldsymbol{s}$, which is found by unwrapping each 2D speckle image into a vector. The length of $\boldsymbol{s}$ is thus dim($\boldsymbol{s}$) = $g_x \cdot g_y$, where $g_x$ and $g_y$ are the number of detector pixels along the $x$ and $y$ dimensions of our two dimensional speckle images, and dim(·) indicates vector length (Supplementary Figure S1). The number of rows in $\boldsymbol{H}$ is set to the output key length dim($\boldsymbol{k}$) = dim($\boldsymbol{s}$) $/c$, $c \geq 1$, where $c$ is a whitening reduction factor estimated by considering the amount of correlation based on speckle size and probe geometry, as well as the deviation of the random process from a uniform random process. Mathematically, $1/c$ defines the size of the subspace that each speckle vector is sparsely projected into. In practice, an example speckle vector $\boldsymbol{s}$ is processed as $c$ is slowly increased until the output key $\boldsymbol{k}$ passes all Diehard and NIST randomness tests, indicating $\boldsymbol{k}$ is a sufficiently random key set for most applications of interest.

A second important parameter associated with matrix $\boldsymbol{H}$ is its measure of sparsity $\varrho$, which gives the density of its non-zero matrix entries. An optimal value of $\varrho$ is selected to balance desired whitening, output noise and digital memory capabilities. For highly biased sources, an ideal value of $\varrho$ is 0.5. However, such a large density of ones both leads to a computationally challenging matrix operation for typical key sizes (~$10^6$ bits). Given an already pseudo-random speckle source, we find a much smaller density of $\varrho \approx 0.001$ is sufficient to generate keys that pass all statistical tests of randomness. A final important parameter is the code rate used for error correction, which sets the rough percentage of processed bits that will eventually form the secret key. As detailed in Section 3, this rate is currently set at 3.5%.

| Parameter | Variable | Experimental Value |
|---|---|---|
| # sensor pixels (8-bit) | $g = g_x \cdot g_y$ | 5.03x $10^6$ |
| Raw speckle vector length | dim($\boldsymbol{s}$) | 4.03 x $10^7$ |
| Whitening reduction factor | $c$ | 5 |
| Output key vector length | dim($\boldsymbol{k}$) = dim($\boldsymbol{s}$)/$c$ | 2.40 x $10^6$ |
| Sparse matrix density of 1's | $\varrho$ | 0.0001 |
| Number of captured speckle images | $n$ | 4300 |
| Error correction code rate | $\kappa$ | 0.035 |

**Supplementary Table S3 | Experimental parameters**. List of variables and their associated numerical values used for experimental ROSS demonstration.

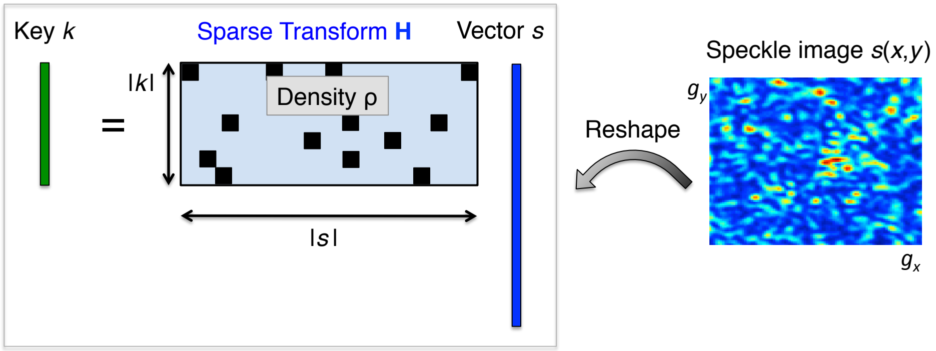


**Supplementary Figure S1 | The digital whitening operator *H*.** The sparse binary random matrix ***H*** converts speckle input ***s*** into key ***k*** via matrix multiplication. ***s*** is formed from reshaping a 2D speckle image into a 1D vector. A properly designed matrix ***H*** will transform a correlated, exponentially distributed speckle vector ***s*** towards an uncorrelated, uniformly distributed key vector ***k***. Typical sizes associated with the above operations are listed in Supplementary Table S3.

The matrix equation $\boldsymbol{k} = \boldsymbol{Hs}$ forms an ideally random key ***k*** given two important conditions. First, this proposed randomness extraction method is efficient, but not optimal, for any ***s*** following a Hidden Markov Process (HMP) [10]. As discussed in [11], ***s*** will follow an HMP if a Cauchy-Lorentz modulation mask is placed at the scatterer's back surface (although such a mask was not used in our tests). Second, ***H*** must be "random" in the sense that each of its matrix elements should be uncorrelated. However, as already noted each device does not require a unique ***H*** – the proposed ROSS protocol remains information-theoretically secure even if we assume the same matrix ***H*** is publically known.

## Supplementary Section 3: Fuzzy Commitment

Fuzzy commitment, also referred to as fuzzy extraction, is a broad class of cryptographic theory. For the sake of clarity, we here only discuss our specific implementation of this general procedure, in terms that a non-expert in cryptography may hopefully understand. Additional details may be found in [12-15].

As noted in the text, fuzzy commitment enables the secure application of noisy yet random measurements to a cryptographic protocol. For example, a biometric measurement such as a fingerprint may be used to gain access to a building, even if the fingerprint is not read in exactly the same fashion as when the user was registered for access. In the case of the ROSS device, noise is introduced between two attempted readings of the same key ***k***, which we would like to identify as a matched pair. The first time we generate ***k*** corresponds to your fingerprint's registration, while any subsequent generation corresponds to a later attempt to gain building access.

Two insights help explain fuzzy commitment's success: forward error correction [16], and the one-time pad [17]. Error correction is typically applied to a vector of $n$ bits, ***k***, to remove any flipped bits that may have been introduced to ***k*** after it has been transmitted over a noisy channel,

for example. This is accomplished by first encoding $\boldsymbol{k}$ into a codeword $\boldsymbol{c} = \boldsymbol{E}[\boldsymbol{k}]$, where $\boldsymbol{c}$ is a longer stream of $m > n$ bits and $\boldsymbol{E}$ is the encoding operation. Next, through whatever physical process, noise is introduced to $\boldsymbol{c}$ to turn it into $\boldsymbol{c'} = \boldsymbol{c} + \boldsymbol{n}$, where $\boldsymbol{n}$ is a vector of noise. This noise can be removed in a final decoding step, where if the noise is below a certain threshold, we find $\boldsymbol{k} = \boldsymbol{D}[\boldsymbol{c'}]$, where $\boldsymbol{D}$ is the decoding operation. Many choices for $\boldsymbol{E}$ and $\boldsymbol{D}$ exist. Repetition coding is a simple example: $\boldsymbol{E}$ can create a codeword $\boldsymbol{c}$ that is e.g. 5 times longer than $\boldsymbol{k}$ by repeating each bit in $\boldsymbol{k}$ five times (i.e., $m = 5n$). $\boldsymbol{D}$ can then look at each group of 5 repeated bits in the noisy $\boldsymbol{c'}$ and select the most frequent bit of each group to reform $\boldsymbol{k}$, which will be successful if the noise is not significant enough to flip 3 or more of 5 the bits within each group of 5 repeated bits.

Fuzzy commitment carries out the above process to check if a secret key $\boldsymbol{k}$ matches a different (but hopefully similar) secret key $\boldsymbol{k'}$, without revealing any information about either key to an attacker. This matching problem is unique from the transmission of a vector over a noisy channel that we just discussed. Since there are two vectors to compare, it is clear that subtracting $\boldsymbol{k'}$ from $\boldsymbol{k}$ is a good first step to reveal any errors. Subtraction is typically achieved with an XOR operation ($\oplus$). For example, we can naively execute our noisy fingerprint matching example by first encoding the binary representation of your fingerprint $\boldsymbol{k}$ as $\boldsymbol{c} = \boldsymbol{E}[\boldsymbol{k}]$, and saving the result. When your fingerprint is read for building access a second time as $\boldsymbol{k'}$, we can also encode it as $\boldsymbol{c'} = \boldsymbol{E}[\boldsymbol{k'}]$. We can then subtract this new codeword $\boldsymbol{c'}$ from the saved codeword $\boldsymbol{c}$ and used decoding to correct any flipped bits. If the decoded sequence contains all zeros, then the fingerprints match, since we'd expect $\boldsymbol{D}[\boldsymbol{c}\text{-}\boldsymbol{c'}] = \boldsymbol{k}\text{-}\boldsymbol{k'} = \boldsymbol{0}$. Otherwise, there was either too much noise to match $\boldsymbol{k'}$ with the correct key $\boldsymbol{k}$, or the fingerprints are simply not from the same user.

There are two problems with the above simple protocol. First, any attacker knows immediately how to access the building – the all-zeros vector $\boldsymbol{0}$ will be the result of any successful attempt at entry, so the system can be easily fooled. Second, the above protocol requires the system to save $\boldsymbol{c}$ directly, which an attacker might be able to gain access to and then directly determine the secret $\boldsymbol{k}$ from. These problems are solved with the introduction of a new important concept – the witness, $\boldsymbol{w}$. We form the witness by splitting the binary representation of your registered secret fingerprint into two vectors. The first random vector will remain the secret key $\boldsymbol{k}$, while the second random vector is the witness $\boldsymbol{w}$ and will contain more bits than $\boldsymbol{k}$, but is qualitatively the same (ideally, both contain uncorrelated random bits). Fingerprint registration now consists of two steps. First, the secret key segment $\boldsymbol{k}$ is encoded into codeword $\boldsymbol{c} = \boldsymbol{E}[\boldsymbol{k}]$, just like before. Second, the witness segment $\boldsymbol{w}$ will be used to securely *hide* the codeword with an XOR operation: $\boldsymbol{b} = \boldsymbol{c} \oplus \boldsymbol{w}$. Assuming $\boldsymbol{w}$ is ideally random, this operation is equivalent to performing one-time pad encryption - a simple scheme proven to be information-theoretically secure [17]. Thus, the blob $\boldsymbol{b}$ will contain no useful information about $\boldsymbol{c}$. The system can save $\boldsymbol{b}$ in digital memory with the knowledge that $\boldsymbol{c}$ is highly secure, in a cryptographic sense, from any attack.

When you attempt to gain building access at a later time, your fingerprint again must be split into two segments, $\boldsymbol{k'}$ and $\boldsymbol{w'}$. Now, the "noisy" witness $\boldsymbol{w'}$ is the only quantity of interest. First, $\boldsymbol{w'}$ is used to *unhide* an estimate of the codeword with an XOR: $\boldsymbol{c'} = \boldsymbol{b} \oplus \boldsymbol{w'}$. Since errors are introduced between forming $\boldsymbol{w}$ and $\boldsymbol{w'}$ from the two different fingerprints, it is usually not possible to recover the original codeword $\boldsymbol{c}$ exactly. Error correction decoding may now remove any bits flipped between $\boldsymbol{c}$ and $\boldsymbol{c'}$: $\boldsymbol{k} = \boldsymbol{D}[\boldsymbol{c'}]$. If the induced errors are below a certain threshold, the secret key $\boldsymbol{k}$ can be recovered exactly, and the system may now grant building access.

Extending these concepts to enable our ROSS device to operate with noisy bits is direct. The first time we create a ROSS key corresponds to registration of an initial fingerprint. We split up this ROSS key into a secret key $\boldsymbol{k}$ and a longer witness $\boldsymbol{w}$. $\boldsymbol{k}$ may be immediately used in any

cryptographic protocol. It will remain physically secure if it is never stored in any digital memory device (volatile or non-volatile). We can instead digitally store an information-theoretically secure blob $\boldsymbol{b}$ to hide the key $\boldsymbol{k}$ until a later time when we'd like to use it again. The same ROSS device is required at a later time to produce a witness $\boldsymbol{w'}$ that is similar enough to the original witness $\boldsymbol{w}$ to enable accurate "unhiding" of key $\boldsymbol{k}$. In our experiments we set the size of one secret key $\boldsymbol{k}$ at 256 bits. The longer witness $\boldsymbol{w}$ is 7.2 kilobytes. Each pixel on our digital detector records an 8-bit value (i.e., a number between 0 and 255), and we maintain the witness $\boldsymbol{w}$ as a sequence of such 1-byte values. We first encode the key $\boldsymbol{k}$ into a 7.2 kilobit codeword $\boldsymbol{c}$ using a (255, 9) Hamming scheme [16], working over 9-bit blocks. Then, to remove additional errors caused by global intensity fluctuation of the laser and detector setup, we first transfer $\boldsymbol{c}$ from binary alphabet (0,1) to the alphabet (63, 191) (i.e., every zero is replaced with 63, and every 1 with 191). Instead of forming blob $\boldsymbol{b}$ with a conventional XOR, we add $\boldsymbol{c}$ and $\boldsymbol{w}$ modulo 255: $\boldsymbol{b = (c + w) \bmod 255}$.

The ROSS device's second measurement produces a noisy witness $\boldsymbol{w'}$. This is identical to the second fingerprint measurement in our previous example. We can use $\boldsymbol{w'}$ to access the secret key $\boldsymbol{k}$ hidden within the digitally saved blob $\boldsymbol{b}$ following three steps. First, we subtract $\boldsymbol{w'}$ from $\boldsymbol{b}$ modulo 255 to create a new codeword: $\boldsymbol{c' = (b - w') \bmod 255}$. This subtraction is equivalent to our fingerprint example's second XOR operation, now performed byte-wise instead of bit-wise. Second, we threshold our new codeword formed of bytes to a codeword formed of bits, $\boldsymbol{c_t'}$: $\boldsymbol{c_t' = 0}$ if $\boldsymbol{0 \leq c' < 128}$, and $\boldsymbol{c_t' = 1}$ otherwise. This threshold operation offers us a 64 bit threshold of error when comparing each bit of $\boldsymbol{w}$ to $\boldsymbol{w'}$, thus minimizing intensity fluctuation effects. Third, we complete our error correction with (255, 9) Hamming decoding: $\boldsymbol{k = D[c_t']}$. This typically recovers the original secret key $\boldsymbol{k}$ error-free, allowing it to be again used in any cryptographic protocol. However, no information about $\boldsymbol{k}$ was digitally saved in this cryptographic pipeline. Its physically security is maintained so long as it never enters volatile or non-volatile digital memory.

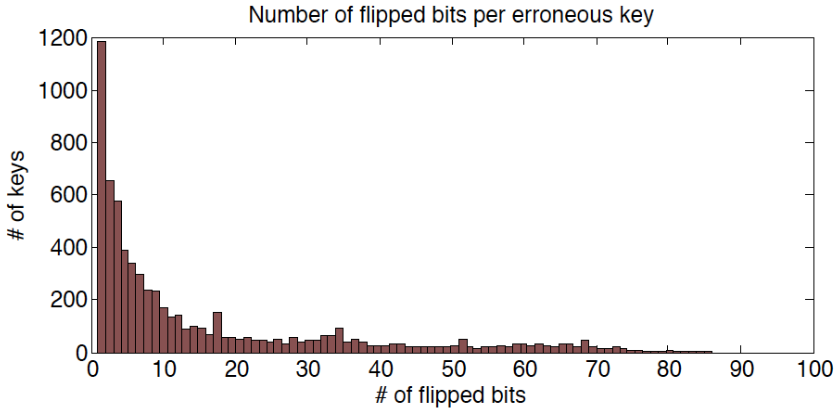


**Supplementary Figure S2 | Histogram of key errors.** Of the 1.43 x $10^6$ keys tested for errors after 24 hours, approximately $10^5$ keys exhibited at least one error. This histogram displays the number of flipped bits per erroneous 256-bit key created in our experiment.

## Supplementary Section 4: Remaining Key Error

Our fuzzy commitment scheme removes a significant number of errors from a final key. On the order of 10-20% of the bits have flipped before error correction. However, error correction is not perfect. Sometimes errors build up heavily within a sequence that is longer than the code block length, preventing their removal. When this occurs, our key recovery procedure fails, and a new key read attempt must be executed.

Supplementary Figure S2 shows the distribution of observed key errors when attempting to access our set of 1.43 million keys after waiting a period of 24 hours. This histogram does not include the ~1.3 million keys that we recover error-free. Only several thousand keys that exhibited at least one flipped bit are shown for graphical clarity. Approximately 10% of the erroneous keys include only one flipped bit – it is much more common to see several bits fail within the same key.

## Supplementary Section 5: Physical security

The security benefits of storing randomness within a volumetric scattering medium, as opposed to digital memory, are of course specific to the type of attack used to probe the device. Here, we examine what type of physical attack our ROSS device must protect against. To begin, it is currently extremely challenging, and perhaps impossible, to accurately reproduce a disordered 3D volume at optical wavelength-scale resolution. Thus, an evesdropper Eve will *not* be able to simply steal and replace a given ROSS with a replica. By periodically verifying the authenticity of the devices they hold through probing with randomly selected SLM patterns $\boldsymbol{p}$, a ROSS user can effectively guard against such a "replica switching" attack. These authenticity checks may also verify if any attempt has been made to maliciously alter the scatterer. Furthermore, it is possible to prevent attempts to probe or alter any required digital circuitry by embedding this circuitry within the ROSS device's scattering medium. Attempts to gain access to any embedded electronics will irreversibly alter the medium's scattering response and thus render the device inoperable.

Thus, it is immediately clear that unlike e.g. a USB device, the ROSS setup cannot be easily probed or copied physically. Instead, it must primarily defend against attackers who somehow have a limited amount of time to quickly characterize its stored contents. This type of "copy" attack is also clearly an issue with USB storage. The ROSS device's security may then be measured in relation to *how long* it would take Eve to extract any useful information from a stolen device. In its current form, the simple ROSS device has a functional lifetime of approximately 50 hours, which is significantly longer than any digital storage mechanism.

With a temporarily stolen ROSS device and control over the SLM display, Eve can mathematically copy its stored random contents. To do so, she must determine the scatterer's structure by recording its optical response to all orthogonal display patterns. This is equivalent to mathematically cloning the transmission matrix $\boldsymbol{T}$, which is of interest in scattering and time-reversal experiments [18]. By characterizing and digitally storing $\boldsymbol{T}$, Eve can later access any key she desires by first monitoring for what SLM pattern $\boldsymbol{p}$ is currently being used, and then digitally computing $\boldsymbol{k} = |\boldsymbol{T}\boldsymbol{p}|^2$. Note that such an attack will require Eve to measure all elements of $\boldsymbol{T}$ (i.e., since each key $\boldsymbol{k}$ depends upon the entire scattering structure, not just one segment). An incomplete matrix will not produce an effective estimate of $\boldsymbol{k}$, since $\boldsymbol{T}$'s randomness ensures that it exhibits a full rank.

We will begin with the assumption that full characterization of ***T*** is possible by probing the scatterer by turning one SLM pixel "on" at a time, as performed in [18]. This is a generous assumption since it assumes ***T*** may somehow be recovered from intensity-only measurements without detecting the complex optical field, which has yet to be demonstrated. Specifically, this assumption reduces the scattering inversion process to a linear problem. As the above key generation equation includes a squaring operation due to the measurement of optical intensity, the problem is certainly not linear, but we will give the attacker the benefit of the doubt. We also assume image capture at 1 frame per second, which is currently shorter than the lower exposure time limit of approximately 2 seconds required to prevent scatterer heating and speckle pattern decorrelation. Scatterer heating is caused by both a high illumination beam intensity as well as sensor heating during rapid readout. Decorrelation from a sub-second key readout rate currently leads each recorded speckle pattern to change into a nearly uncorrelated pattern within minutes.

As described in [19], ***T*** contains on the order of $10^8$ rows, while the current device's SLM contains 2 x $10^6$ pixels. Based upon these parameters and the above two modest assumptions, Eve will require 2 x $10^6$ seconds, or approximately 23 days, to completely measure an ideal stolen device's scattering matrix ***T***. Assuming Eve can attach some cooling mechanism to probe the device at the SLM's maximum 15 frames-per-second rate, CPUF characterization will still require roughly 2 days. This estimate leads to our suggested cloning time of several days (~50 hours) included in the paper. While it is reasonable to assume that Alice or Bob will notice their device missing over such a long period, we aim future work at extending this device lifetime.

The above argument assumes that Eve does not have access to any display pattern ***p*** that has been or will be used to create a key. Assuming the PDLC film is not reset, Eve may use any known ***p*** to directly recover its corresponding keys, thus rendering the ROSS device completely insecure. Deleting each ***p*** after its use, not saving any ***p*** that will be used in the future, and reconfiguring the PDLC film whenever possible will clearly help prevent such an attack. When ***p*** must be digitally stored, two-factor authentication is a well-known tool to enhance the security of any cryptographic system. Password-protecting any used pattern ***p*** will clearly offer additional security against an attacker from quickly extracting choice keys from a stolen ROSS device.

Finally, once the key is read from the ROSS device and digitized, a number of computer-side attacks may still reveal its contents to Eve. While beyond the scope of this paper, there is a growing body of work surrounding the development of efficient digital protocols to safely take advantage of the physical security offered by PUF setups [20-24].

## Supplementary Material References:


1. Marsaglia, G. *DIEHARD: A battery of tests of randomness.*<http://stat.fsu.edu/pub/diehard> [Accessed September 15th, 2013] (1996).
2. Rukhin, A. *et al.* A statistical test suite for random and pseudorandom number generators for cryptographic applications. (*Special Publication* 800-22 *Revision 1*, *National Institute of Standards and Technology, 2008*); available at <http://csrc.nist.gov/publications/PubsSPs.html>.
3. Kim, S. J., Umeno, K. & Hasegawa, A. Corrections of the NIST statistical test suite for randomness. arXiv:nlin.CD/ 0401040v1 (2004).
4. Uchida, A. *et al.* Fast physical random bit generation with chaotic semiconductor lasers.*Nat. Photonics* **2**, 728–732 (2008).
5. Kanter, I., Aviad, Y., Reidler, I., Cohen, E. & Rosenbluh, M. An optical ultrafast random bit generator. *Nat. Photonics* **4**, 58–61 (2010).
6. von Neumann, J. Various techniques used in connection with random digits. *Applied Math Series* **12**, 36–38 (1951).
7. Peres, Y. Iterating Von Neumann's procedure for extracting random bits. *Ann. Stat.* **20**(1), 590-597 (1992).

8. Nisan, N. & Zuckerman, D. Randomness is Linear in Space. *J. Comput. Syst. Sci.* **52**(1), 43-52 (1996).
9. Elias, P. The efficient construction of an unbiased random sequence. *Ann. of Math. Stat.* **43**(3), 865-870 (1972).
10. Zhou, H. & Bruck, J. Linear extractors for extracting randomness from noisy sources.*Proceedings of the 2011 IEEE International Symposium on Information Theory*,1738–1742; doi:10.1109/ISIT.2011.6033845 (2011).
11. Horstmeyer, R., Chen, R., Judkewitz, B. & Yang, C. Markov speckle for efficient random bit generation. *Opt. Express* **20**, 26394–26410 (2012).
12. Juels, A. & Wattenberg, M. A fuzzy commitment scheme. *6th ACM Conf. on Computer and Communications Security*, ACM Press, 28-36 (1999).
13. Dodis, Y., Reyzin, M. & Smith, A. Fuzzy extractors: How to generate strong keys from biometrics and other noisy data. *Proc. EUROCRYPT 2004 LNCS* **3027**, 523–540 (2004).
14. Dodis Y., and Smith, A. Correcting errors without leaking partial information. *Proc. ACM Symposium on Theory of Computing*, 654-663 (2005).
15. Tuyls, P., Skoric, B. & Kevenaar, T. *Security with Noisy Data* (Springer-Verlag, London,2007).
16. Cover, T. M. & Thomas, J. A. *Elements of Information Theory* (John Wiley and Sons, Inc., 1991).
17. Shannon, C. Communication theory of secrecy systems. *Bell Syst. Tech. J.* **28**, 656–715(1949).
18. Popoff, S., et al. Measuring the transmission matrix in optics: an approach to the study and control of light propagation in disordered media. *Phys. Rev. Lett.* **104**(10), 100601 (2010).
19. Horstmeyer, R., Judkewitz, B., Vellekoop, I. M., Assawaworrarit, S. & Yang, C. Physical key-protected one-time pad. Scientific Reports **3**, 3543 (2013).
20. Lim, D. et al. Extracting secret keys from integrated circuits. *IEEE Trans. VLSI Syst.* **13**,1200–1205 (2005).
21. Gassend, B. et al. Controlled physical random functions and applications. *ACM Trans. Inform. Syst. Se.* **10**, 15–27 (2008).
22. Yu, M. & Devadas, S. Secure and robust error correction for physical unclonable functions.*IEEE Des. Test Comput.* **27**, 48–65 (2010).
23. Beckmann, N. & Potkonjak, M. Hardware-based public-key cryptography with public physically unclonable functions. In *Information Hiding 2009*, DOI:10.1007/978-3-642-04431-1_15 (2011).
24. Ruhrmair, U. and van Dijk, M. On the practical use of physical unclonable functions in oblivious transfer and bit commitment protocols. J. Cryptogr. Eng. **3**:17-28 (2013).
